# Supplementary material for: Partial Force Control of Constrained Floating-Base Robots
Source: arXiv:1410.4426 source file (2014-10-16)
Supplement: Supplementary file 1 [file A-appendix.tex]

%!TEX root =  ../PartialForceCtrl.tex
%\section{Appendix}
\label{sec:appendix}
%We want to prove that \dots.

%Starting from the assumptions that $\rank{J_s U^\T} = 6$ and $\tau$ takes the form \eqref{eq:torque_sol}, we show that:
%\begin{enumerate}
%\item $\rank{Z_s S^\T}=n+6-k_s$
%\item $\ddot{q} = z^*$;
%\item 
%\end{enumerate}
We can interpret the proposed reformulation as follows. 
Rather than solving the constraints (i.e. the system dynamics \eqref{const_under_dyn}) numerically, we find an analytical solution and we substitute it in the cost functions. 
This allows us to pass from a constrained problem in $y \in \Rv{2n+6-k}$ to an unconstrained problem in $\hat{y}^\T = \mat{z_c^\T & \lambda_f^\T & \tau_0^\T} \in \Rv{n}$.
This analytical solution is particularly convenient because it is sparse in $\ddot{q}$ and $f_f$, which are the only variables appearing inside the cost functions.
The proposed analytical solution of \eqref{const_under_dyn} is:
\begin{equation} \label{eq:tau_change_var} \begin{split}
\ddot{q} =& J_c^\pinv c_c + Z_c z_c \\
f_f         =& T_f \lambda_f + Y_f Y_f^\T \tilde{f}_f \\
f_s        =& J_s^{\T \pinv} ((I-S^\T (Z_s S^\T)^\pinv Z_s) (M (J_c^\pinv c_c + Z_c z_c) + h \\
               & - J_f^\T T_f \lambda_f) - S^\T Z_{ss} \tau_0) + Y_s Y_s^\T \tilde{f}_s \\
\tau       =& (Z_s S^\T)^\pinv Z_s (M(J_c^\pinv c_c + Z_c z_c) + h \\
             & -J_f^\T T_f \lambda_f) + Z_{ss} \tau_0,
\end{split}\end{equation}
\begin{equation} \label{eq:tau_change_var} \begin{split}
\mat{\ddot{q} \\ f_f  \\ f_s \\ \tau}
=
\mat{  Z_c                                          &                     0                                 &    0        \\
          0                                              &                   T_f                                &    0         \\
          J_s^{\T \pinv} N_{ss} M Z_c    & -J_s^{\T \pinv} N_{ss} J_f^\T T_f    &  -J_s^{\T \pinv} S^\T Z_{ss} \\
          (Z_s S^\T)^\pinv Z_s M Z_c    & -(Z_s S^\T)^\pinv Z_s  J_f^\T T_f   &  Z_{ss}   }
\mat{z_c \\ \lambda_f \\ \tau_0}
+
\mat{J_c^\pinv c_c \\
        Y_f Y_f^\T \hat{f}_f \\
        J_s^{\T \pinv} N_{ss} (MJ_c^\pinv c_c + h) + Y_s Y_s^\T \hat{f}_s \\
        (Z_s S^\T)^\pinv Z_s (MJ_c^\pinv c_c + h)}
\end{split}\end{equation}
%This mapping actually represents an analytical solution of the system dynamics \eqref{const_under_dyn}.
%We can then remove \eqref{const_under_dyn} from the optimization and get an unconstrained problem with only $n$ variables.
%Since the cost functions depend only of $\ddot{q}$ and $f_f$ we do not need to compute $M$ (we would if we had a cost on $\tau$ or $f_s$).
If no cost function depends on both $\ddot{q}$ and $f_f$ --- as we assumed --- we can split the resulting optimization into two independent problems in $z_c$ and $\lambda_f$, respectively.

It is trivial to show that \eqref{eq:tau_change_var} encodes the solutions of the constraint $J_c \ddot{q} = c_c$.
It is not trivial instead to prove it for the multibody dynamics constraint.
We project the dynamics into three orthogonal subspaces of $\Rv{n+6}$ by using these basis: i) $V_s$, ii) $Z_s V_{fs}$ and iii) \mbox{$Z_s Z_{fs} (= Z_c)$}.
Since the union of these subspaces spans $\Rv{n+6}$, the three projected dynamics are equivalent to the original dynamics.
It is then sufficient to prove that \eqref{eq:tau_change_var} is a solution of the three projected dynamics.
To do that we must exploit our assumption that $\rank{J_s \bar{S}^T} = 6$, which implies that $Z_s^\T S^\T$ is full rank.
For the sake of brevity we report hereafter only the proof for the projection with $Z_s Z_{fs}$:
\begin{equation} \begin{split} \label{eq:dyn_proj}
Z_{fs}^\T Z_s^\T(M \ddot{q} + h) - \underbrace{Z_{fs}^\T Z_s^\T J_c^\T}_0 f = Z_{fs}^\T Z_s^\T S^T \tau,
\end{split} \end{equation}
We substitute $\ddot{q}$ and $\tau$ with their expression from \eqref{eq:tau_change_var}:
\begin{equation*} \begin{split} 
&Z_{fs}^\T Z_s^\T(M(J_c^\pinv c_c + Z_c z_c ) + h) = \\
&Z_{fs}^\T \underbrace{Z_s^\T S^\T (Z_s^\T S^\T)^\pinv}_I Z_s^\T(M(J_c^\pinv c_c + Z_c z_c) + h - J_f^\T T_f \lambda_f)
\end{split} \end{equation*}
With some simplifications we can then show that this equation is always satisfied.
