# Supplementary material for: Partial Force Control of Constrained Floating-Base Robots
Source: arXiv:1410.4426 source file (2014-10-16)
Supplement: Supplementary file 3 [file A-appendixOld.tex]

%!TEX root =  ../PartialForceCtrl.tex
%\section{Appendix}
\label{sec:appendix}
In this appendix we want to prove that:
\begin{equation*}
\rank{J_s \bar{S}^\T} = 6 \quad \equiv \quad \rank{S Z_s} = n+6-\hat{k}_s
\end{equation*}
%where 
%$S = \mat{0_{n\times 6} & I_{n\times n}} \in \mathbb{R}^{n\times (n+6)}$ is the joint selection matrix,
%$\bar{S} = \mat{I_{6\times 6} & O_{6\times n}}$ is the base selection matrix, 
%$J_s \in \R{k_s}{n+6}$ is the supporting constraint Jacobian and
%$Z_s \in \R{n+6}{n+6-\hat{k}_s}$ is a base of the nullspace of $J_s$.
Before starting the demonstrations, we introduce the singular value decomposition of $J_s$:
\begin{equation*}
J_s = \underbrace{\mat{U_s & \bar{U}_s}}_U \mat{\Sigma_s & 0 \\ 0 & 0} \underbrace{\mat{ \bar{Z}_s^\T \\ Z_s^\T }}_Z = U_s \Sigma_s \bar{Z}_s^\T,
\end{equation*}
where $Z_s \in \mathbb{R}^{n+6 \times n+6-\hat{k}_s}$ is an orthonormal basis of the \emph{nullspace} of $J_s$, 
and $U_s \in \mathbb{R}^{n+6 \times \hat{k}_s}$ is an orthonormal basis of the \emph{range} of $J_s$.
We start by proving that the first condition implies the second one.
Since $\rank{J_s \bar{S}^\T} = \rank{\bar{Z}_s^\T \bar{S}^\T}$ and $\rank{\bar{Z}_s}=\hat{k}_s$ we have that:
\begin{equation*}
\rank{\bar{Z}_s} = \rank{\mat{\bar{S} \\ S}\bar{Z}_s} = \rank{\mat{\bar{S} \bar{Z}_s \\ S \bar{Z}_s}} = \hat{k}_s
\end{equation*}
Now, since $\rank{\bar{S} \bar{Z}_s}=6$ by assumption, we can infer that $\rank{S\bar{Z}_s}=\hat{k}_s-6$.
Similarly, since $\rank{S}=n$ and $Z$ is orthogonal, we can claim that:
\begin{equation*}
\rank{S^\T} = \rank{Z^\T S^\T} = \rank{\mat{\bar{Z}_s^\T S^\T \\ Z_s^\T S^\T}} = n
\end{equation*}
Since we just showed that $\rank{\bar{Z}_s^\T S^\T}=\hat{k}_s-6$, this implies that $\rank{Z_s^\T S^\T}=n+6-\hat{k}_s$.
This proves that the first condition implies the second one.
We can prove that the second condition implies the first one by means of the same reasoning.

%Since $\rank{S}=n$ and $V$ is orthogonal, we can claim that:
%\begin{equation}
%\rank{V^T S^T} = \rank{\mat{V_1^T S^T \\ V_2^T S^T}} = n
%\end{equation}
%Since $\rank{V_2^TS^T}=n+6-k_s$ by assumption, this implies that $\rank{V_1^T S^T}=k_s-6$.
%Similarly, since $\rank{V_1}=k_s$ we have that:
%\begin{equation}
%\rank{\mat{U \\ S}V_1} = \rank{\mat{UV_1 \\ SV_1}} = k_s
%\end{equation}
%Now, since we already proved that $\rank{SV_1}=k_s-6$, we can infer that $\rank{U V_1}=6$.

%Assume 
%$V = \mat{V_1 & V_2} \in \R{n+6}{n+6}$, 
%$U = \mat{I_{6\times 6} & O_{6\times n}}$ and 
%$S = \mat{0_{n\times 6} & I_{n\times n}} \in \R{n}{n+6}$. 
%Assume also that $V$ is orthogonal.
%We want to prove that this condition:
%\begin{equation}
%\rank{U V_1} = 6,
%\end{equation}
%is equivalent to this condition:
%\begin{equation}
%\rank{S V_2} = n+6-k
%\end{equation}
%We start by proving that the second condition implies the first one.
%Since $\rank{S}=n$ and $V$ is orthogonal, we can claim that:
%\begin{equation}
%\rank{V^T S^T} = \rank{\mat{V_1^T S^T \\ V_2^T S^T}} = n,
%\end{equation}
%Since $\rank{V_2^TS^T}=n+6-k$ by assumption, this implies that $\rank{V_1^T S^T}=k-6$.
%Similarly, since $\rank{V_1}=k$ we have that:
%\begin{equation}
%\rank{\mat{U \\ S}V_1} = \rank{\mat{UV_1 \\ SV_1}} = k
%\end{equation}
%Now, since we already proved that $\rank{SV_1}=k-6$, we can infer that $\rank{U V_1}=6$.
%This proves that the second condition implies the first one.
%To prove that the first condition implies the second one the reasoning is basically the same: 
%\begin{align} 
%\rank{UV_1}=6 \implies \rank{SV_1}=k-6, \\
%\rank{SV_1}=k-6 \implies \rank{S V_2} = n+6-k
%\end{align}
